# Supplementary material for: Traffic incident duration prediction via a deep learning framework for text description encoding
Source: arXiv:2209.08735 source file (2022-09-19)
Supplement: Supplementary file 1 [file appendix.tex]

\clearpage

  \appendix 

This document is accompanying the submission \textit{\titlename}.
The information in this document complements the submission, and it is presented here for completeness reasons. It is not required for understanding the main paper, nor for reproducing the results.
 
\subsection{NSTM model representation}

 \begin{figure}[h]
 \centering
	\includegraphics[width=0.49\textwidth]{Sydney_network_layout_EMME_Centroids.pdf}%scale=0.45
	\caption{North Sydney Transport network layout including the connection of centroids (main entry points of vehicles in the network; marked as circles with blue interior) and permanent traffic count locations (marked in green dots).  }
	\label{Sydney_network_layout_EMME_Centroids}
\end{figure}

 \begin{figure}[h]
%\begin{adjustbox}{width=1\textwidth}
\centering
	\includegraphics[width=0.49\textwidth]{Sydney_network_layout_PTC_stations.pdf}%scale=0.45
	\caption[width=1\textwidth]{Layout of detector traffic flow.}
	\label{Sydney_network_layout_PTC_stations}
%\end{adjustbox}
\end{figure}
 
 \begin{figure}[h]
%\begin{adjustbox}{width=1\textwidth}
\centering
	\includegraphics[width=0.4\textwidth]{SCATS_Control_intersection.pdf}%scale=0.45
	\caption[width=1\textwidth]{Sample representation of a signalised intersection including signal controls, phases, turnings and detectors for vehicle counting per each turning.}
	\label{SCATS_Control_intersection}
%\end{adjustbox}
\end{figure}

\subsection{NSTM - PM peak validation}\label{PM_validation}

The model validation and calibration has been done as well for the PM peak hours as represented in figures below. 

\begin{figure}[h]%[width=0.49\textwidth,align=\centering]
	\centering
%	\subfloat[]{
		\includegraphics[width=0.4\textwidth]{PM_trip_distribution.pdf}%
		\label{PM_OD_adjustment_fig}
%	}\\
\caption{Validation of PM-NSTM model via Trip Length Distribution }
\end{figure}
\begin{figure}[h]%[width=0.49\textwidth,align=\centering]
%		\subfloat[]{
		\includegraphics[width=0.4\textwidth]{NSTM_PM_flow_validation_R2.pdf}%
		\label{PM_R2_fig}
%	}%
		\caption{Validation of the PM-NSTM model with $R^2=0.91$ metric.}
	\vspace{-.3cm}
\end{figure}
 
While the PM peak distribution after calibration indicates a lower number of adjusted vehicles travelling in the network, the trend profile still follows the original profiling of the data set.  In addition \cref{PM_R2_fig} indicates a high $R^2=0.91$ which is a proof of model well calibrated, despite few cases of over and under calibrated traffic counts.

\subsection{NSTM - car arrivals and mean distance travelled}\label{NSTM_distance_car_flow}
One of the outputs of the NSTM model is the total number of arrivals and departures from each area during AM and PM peaks. For modelling a home to destination charging, the number of arriving cars in each urban area is extremely important in order to be able to estimate the total number of EVs that will require charging at specific times. \cref{AM_car_arrivals_by_area} and \cref{PM_car_arrival_by_area} indicates the AM and PM car arrivals for each of the urban Local Governmental Area in our case study which allowed us to identify the top most attractive locations. For example, Dalley is a small catchment, but this area connects two parts of the city through Harbour Bridge. %There is a high number of vehicles ($19.3\%$) arriving within area by travelling approximatively $17.5 km$.​
 \begin{figure}[h]
 \centering
	\includegraphics[width=0.45\textwidth]{AM_car_arrivals_by_area.pdf}
	\caption{NTSM car arrival by area - AM peak.}
	\label{AM_car_arrivals_by_area}
\end{figure}
 \begin{figure}[h]
 \centering
	\includegraphics[width=0.4\textwidth]{AM_distance_travelled_by_area.pdf}
	\caption{NTSM mean distance travelled - AM peak.}
	\label{AM_distance_travelled_by_area}
\end{figure} 
  \begin{figure}[h]
 \centering
	\includegraphics[width=0.45\textwidth]{PM_car_arrival_by_area.pdf}
	\caption{NTSM car arrival by area - PM peak.}
	\label{PM_car_arrival_by_area}
\end{figure}
 \begin{figure}[h]
 \centering
	\includegraphics[width=0.4\textwidth]{PM_distance_travel_by_area.pdf}
	\caption{NTSM mean distance travelled - PM peak.}
	\label{PM_distance_travel_by_area}
\end{figure}
 \subsection{Capacity and loading of 10 most popular EV stations}\label{EV_load}
    \begin{figure}[h]
 \centering
	\includegraphics[width=0.4\textwidth]{Zone_substation_area_selection.pdf}
	\caption{Zone substation area catchment.}
	\label{Zone_substation_area_selection}
\end{figure}
The Zone substation catchment area helped to identify the mapping of EV stations to the regional energy consumption and the analysis of the energy load for the top 10 most popular stations. Findings have revealed that 7 out of these 10 stations are operating at more than $75\%$ of their capacity, which already reveals current EV infrastructure limitation for further EV uptake. 
 \begin{figure}[h]
 \centering
	\includegraphics[width=0.4\textwidth]{Load_of_EV_Stations_Nord_Sydney.pdf}
	\caption{Load and capacity of 10 most popular EV stations.}
	\label{Traffic_flow_fluctuations_in_the_network}
\end{figure}

 \subsection{Energy impact of various scenarios}\label{EV_load}

 \begin{figure*}[ht]
 \centering
	\includegraphics[width=1\textwidth]{2016-2026-2036_raw_results_table.PNG}
	\caption{Raw results for EV-Q model outputs for OD2016, OD15, OD30 aggregated across all stations.}
	\label{2016_2026_2036_raw_results_table}
\end{figure*}

  \begin{figure}[h]
 \centering
	\includegraphics[width=0.45\textwidth]{MWT_N10.pdf}
	\caption{Mean queue variation for 10 plug EV stations.}
	\label{Queue_for_10_plug_stations}
\end{figure}

   \begin{figure}[h]
 \centering
	\includegraphics[width=0.45\textwidth]{TEC_Stations_2.pdf}
	\caption{Energy consumption of all stations vs $EV_p$,}
	\label{TEC_Stations_2}
\end{figure}
